# Supplementary material for: OED: Towards One-stage End-to-End Dynamic Scene Graph Generation
Source: arXiv:2405.16925 source file (2024-05-27)
Supplement: Supplementary file 1 [file X_suppl.tex]

% \clearpage
\setcounter{page}{1}

\begin{figure*}[!hb]
\includegraphics[width=\linewidth]{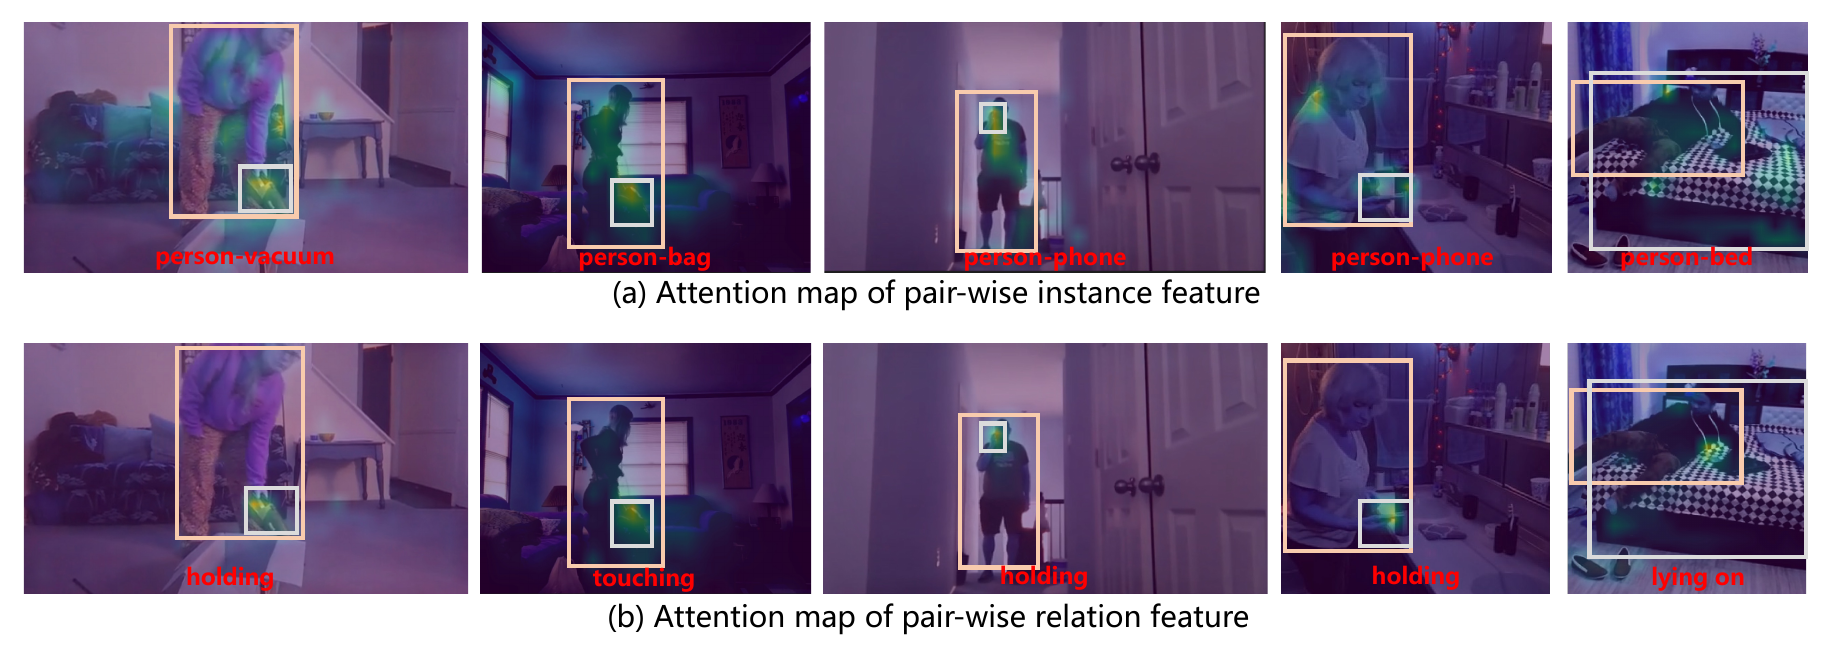}
\caption{Visualization of attention maps of pair-wise instance feature and pair-wise relation feature.}
\label{fig:supp_visual_attn}
\end{figure*}
\begin{table*}[h!]
\captionsetup{font=footnotesize}
% \fontsize{40.5}{13.8}\selectfont

% \setlength{\abovecaptionskip}{0cm} % 调整间距
% \setlength{\belowcaptionskip}{-0.4cm}
\Huge
\centering
\caption{Performance comparison under both Recall and Mean Recall Metrics and Head-body-tail classes with mR@50.}
\resizebox{\textwidth}{!}{
\begin{tabular}{c ccc|ccc|ccc | ccc|ccc|ccc}
\toprule
  & \multicolumn{9}{c|}{With Constraint} & \multicolumn{9}{c}{No Constraints} \\ 
  \cmidrule(lr){2-10} \cmidrule(lr){11-19}
  Method
    &R@10 &R@20 &R50 &mR@10 &mR@20 &mR50  &Head &Body &Tail &R@10 &R@20 &R50 &mR@10 &m20 &mR50  &Head &Body &Tail\\
% \midrule
\midrule

STTran~\cite{cong2021spatial}	&25.2 &34.0 &\underline{36.9} &16.5 &20.8 &22.2 &\underline{39.00} &25.53 &12.78  &24.5 &36.1 &\underline{48.8} &20.9 &29.6 &39.1 &\underline{45.39} &52.32 &26.67 \\
DSG-DETR~\cite{feng2023exploiting} &\underline{30.4} &\underline{34.9} &36.0 &18.0 &21.3 &22.0 &37.91 &\underline{25.84} &12.62 &\underline{32.3} &\underline{40.9} &48.2 &23.6 &30.1 &36.5 &44.76 &\underline{52.65} &21.09 \\
TEMPURA~\cite{nag2023unbiased} &28.0 &33.3 &34.8 &\underline{18.4} &\underline{22.5} &\underline{23.6} &36.53 &23.79 &\underline{18.15} &29.8 &38.0 &46.3 &\underline{24.5} &\underline{33.8} &\underline{43.6} &42.50 &50.66 &\underline{38.86} \\
Ours &\textbf{33.5} &\textbf{40.9} &\textbf{48.9} &\textbf{20.9} &\textbf{26.9} & \textbf{32.9} &\textbf{51.44} &\textbf{36.38} &\textbf{22.72} &\textbf{35.3} &\textbf{44.0} &\textbf{51.8} &\textbf{26.3} &\textbf{39.5} &\textbf{49.5} &\textbf{48.75} &\textbf{56.12} &\textbf{44.89} \\

\bottomrule
\end{tabular}
}
\label{tab:supp_long_tail}
% \vspace{-13pt}
\end{table*}

\begin{figure*}[htpb]
    \includegraphics[width=\linewidth]{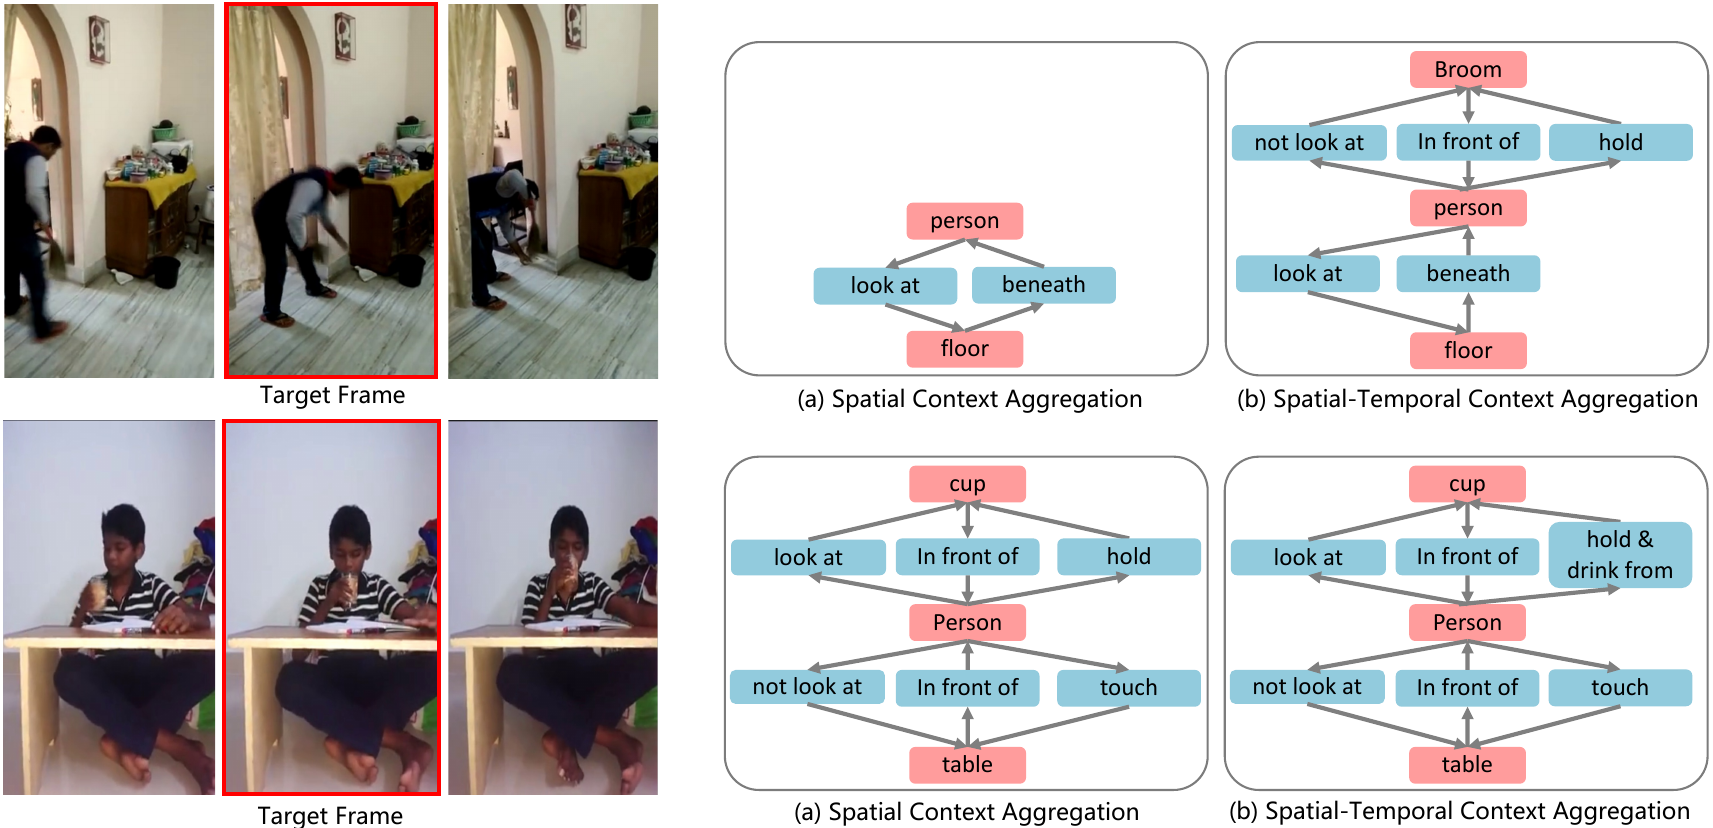}
    \caption{Part of predictions of our Spatial Context Aggregation and Spatial-Temporal Context Aggregation under \textit{with constraint} setting, which match with ground truth.}
\label{fig:supp_scene_graph}
\end{figure*}
Our supplementary material presents long-tail related performance comparison in section~\ref{sec:supp_long_tail} and some qualitative cases to demonstrate different effects of our spatial context aggregation and temporal context aggregation in section~\ref{sec:quali}.

%%%%%%%%%%%%%%%%%%%%%%%%%%%%%%%
\section{Long-tail Problem}
\label{sec:supp_long_tail}
% Visual relations detection is a long-tailed problem. 
% In order to comprehensively evaluate our method, we present a comparison with publicly available SOTA methods under some long-tail related metrics in Tab.~\ref{tab:supp_long_tail}, following TEMPURA~\cite{nag2023unbiased}.
% Our method achieves a notable lead under all metrics.
% Specifically, our approach obtains mR@50 improvements of 9.3\% and 5.9\% over the strongest baseline under \textit{With Constraint} and \textit{No Constraints} settings respectively. 
% Furthermore, we dissect performances across head, body and tail classes with mR@50.
% The comparison shows a significant margin over other methods in all metrics, even though TEMPURA is specifically tailored for the long-tail challenge.

Visual relation detection presents a significant challenge due to its long-tailed distribution. To thoroughly assess our methodology, we conduct a comparison against sota methods that are publicly available in SGDET task, utilizing metrics related to the long-tail issue as detailed in Table~\ref{tab:supp_long_tail}, in line with the approach taken by TEMPURA~\cite{nag2023unbiased}. Our method consistently outperforms across all evaluated metrics, achieving notable improvements in mean Recall@50 (mR@50) by 9.3\% and 5.9\% over the most competitive baseline within the \textit{With Constraint} and \textit{No Constraints} scenarios, respectively.

Additionally, we delve into the performance across different class segments—head, body, and tail—using mR@50 for a more granular analysis. The results demonstrate our method’s superior performance across all metrics, establishing a significant lead over other approaches, despite TEMPURA being specifically designed to address the long-tail challenge.

\section{Qualitative Results}
\label{sec:quali}

\subsection{Spatial Context Aggregation}

As can be seen from Fig.~\ref{fig:supp_visual_attn}, we visualize the decoder attention map for the predicted scene graph. The pair-wise instance heatmaps generated by pair-wise instance decoder highlight both the subject and object area, as shown in Fig.~\ref{fig:supp_visual_attn} (a), meaning that our model reasons for pair-wise instance from a long-range global image context. Meanwhile, as shown in Fig.~\ref{fig:supp_visual_attn}(b), some areas with relatively higher attention weight indicate the relational region in pair-wise relation heatmaps generated by pair-wise relation decoder. It is obvious that the decoder has the ability to find the discriminative part for pair-wise instance and relation information in our one-stage approach.

\subsection{Temporal Context Aggregation}
As illustrated in Fig.~\ref{fig:supp_scene_graph}, we present several scene graph predictions to demonstrate the distinct effects of Temporal Context Aggregation~(TCA). Given a target frame, we attempt to generate scene graphs using our model with only Spatial Context Aggregation~(SCA) and a complete framework incorporating both SCA and TCA. 

SCA can provide sufficient information for relatively static subject-object pairs and predicates with weak or no temporal dependency, as shown in Fig.~\ref{fig:supp_scene_graph}(a), e.g., $<$ cup $-$ in front of $-$ person $>$, $<$person $-$ look at $-$ floor$>$. However, spatial context struggles to handle cases involving blurred subject-object pairs and predicates with strong temporal dependencies. In the first row, the model with only SCA fails to detect the blurred broom. In the second row, the SCA model is unable to recognize the predicate \textit{drink from} due to the lack of temporal dependency. In contrast, our model with Spatial-Temporal Aggregation effectively captures both the temporal dynamics of object motion and the dependency of predicates, resulting in more accurate scene graph prediction, as shown in Fig.~\ref{fig:supp_scene_graph}(b).
