# Supplementary material for: OED: Towards One-stage End-to-End Dynamic Scene Graph Generation
Source: arXiv:2405.16925 source file (2024-05-27)
Supplement: Supplementary file 2 [file supp_fig1_prm.tex]

\begin{figure*}[!t]
    \includegraphics[width=\linewidth]{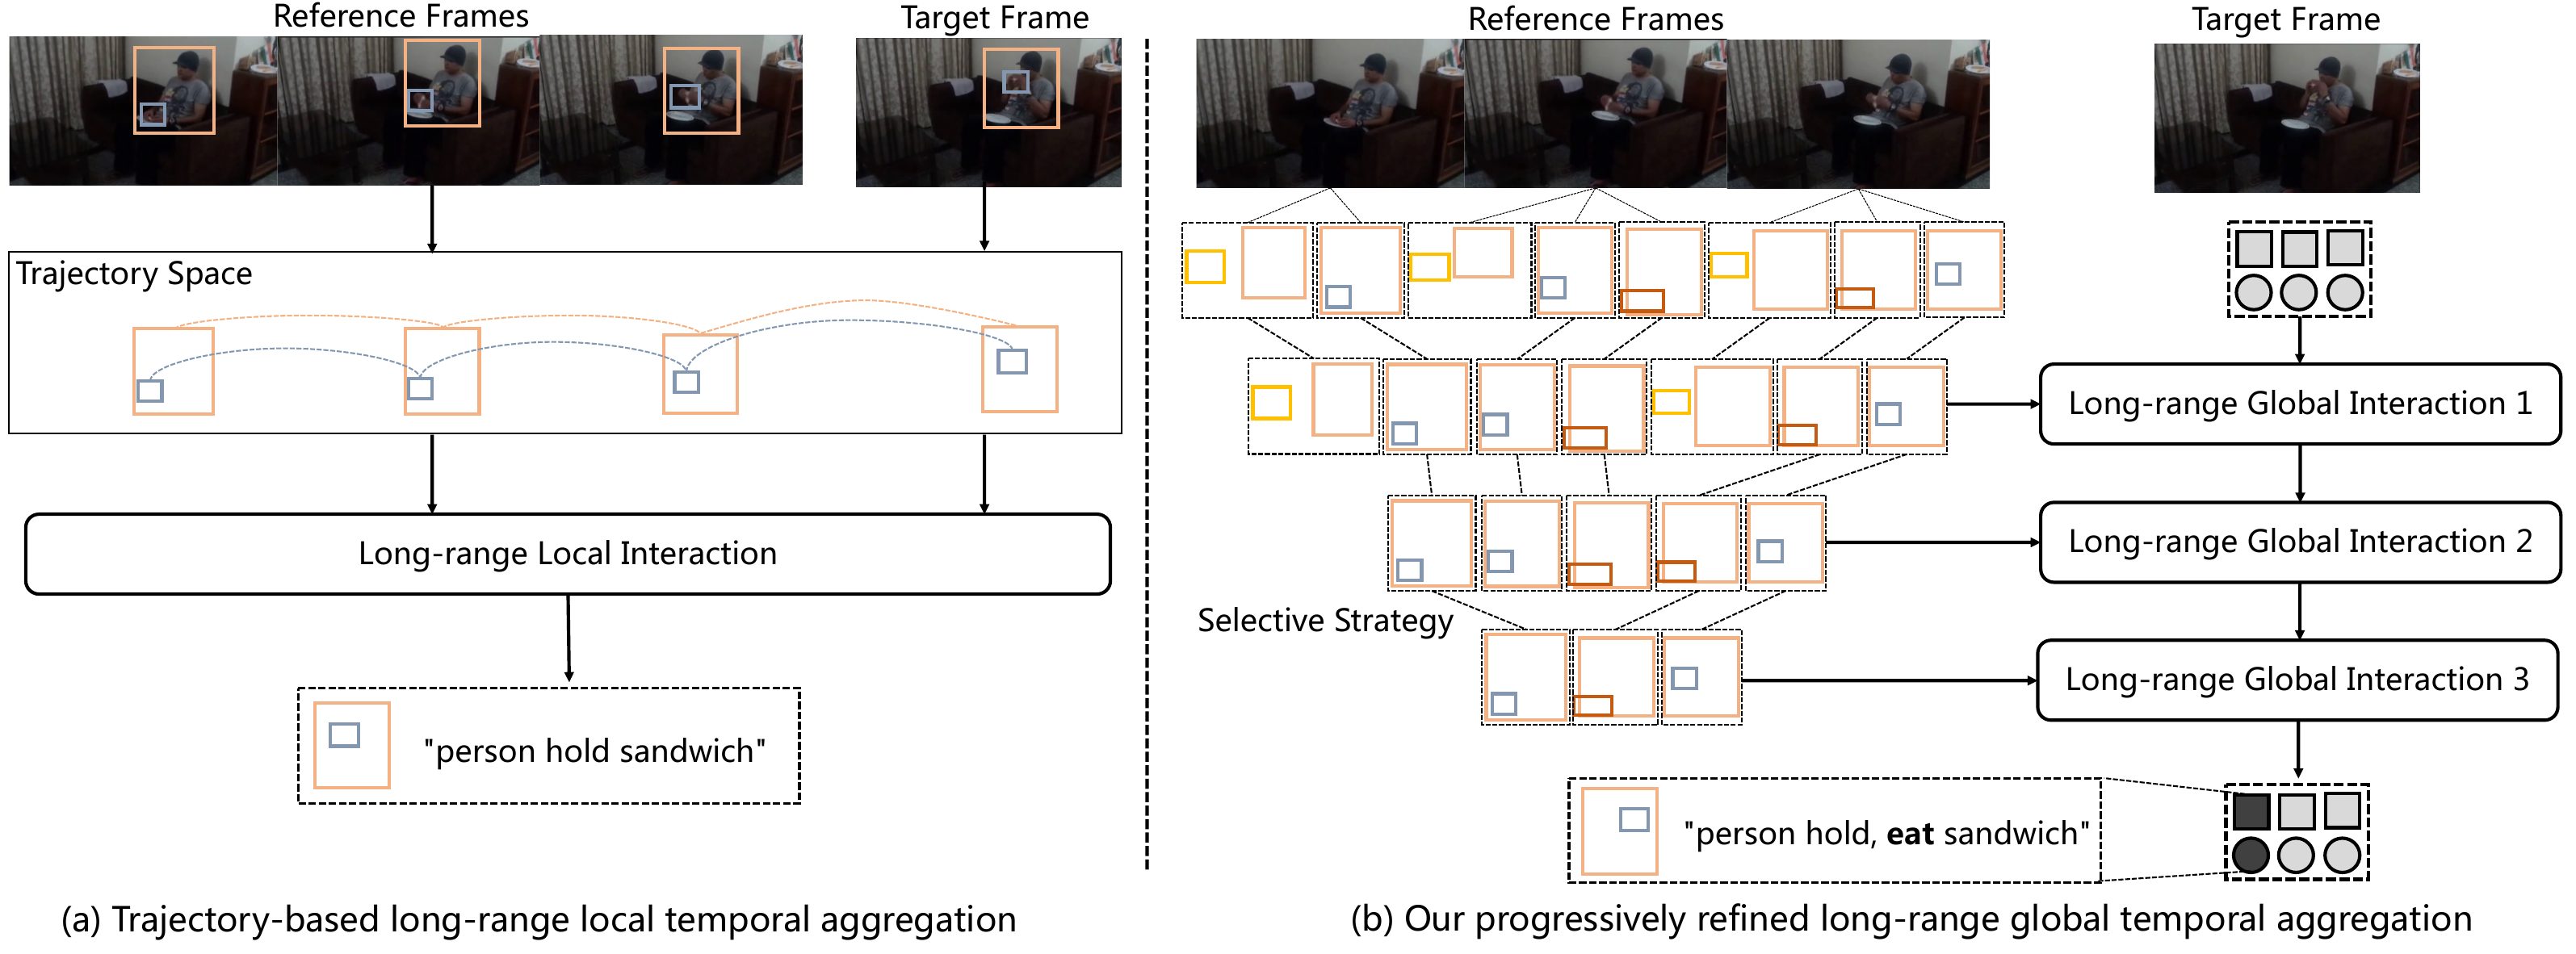}
    \caption{Zoom in Progressively Refined Module.}
\label{fig:supp_prm}
\end{figure*}
