# Supplementary material for: OED: Towards One-stage End-to-End Dynamic Scene Graph Generation
Source: arXiv:2405.16925 source file (2024-05-27)
Supplement: Supplementary file 3 [file supp_fig2_visual_attn.tex]

\begin{figure*}[t]
    \includegraphics[width=\linewidth]{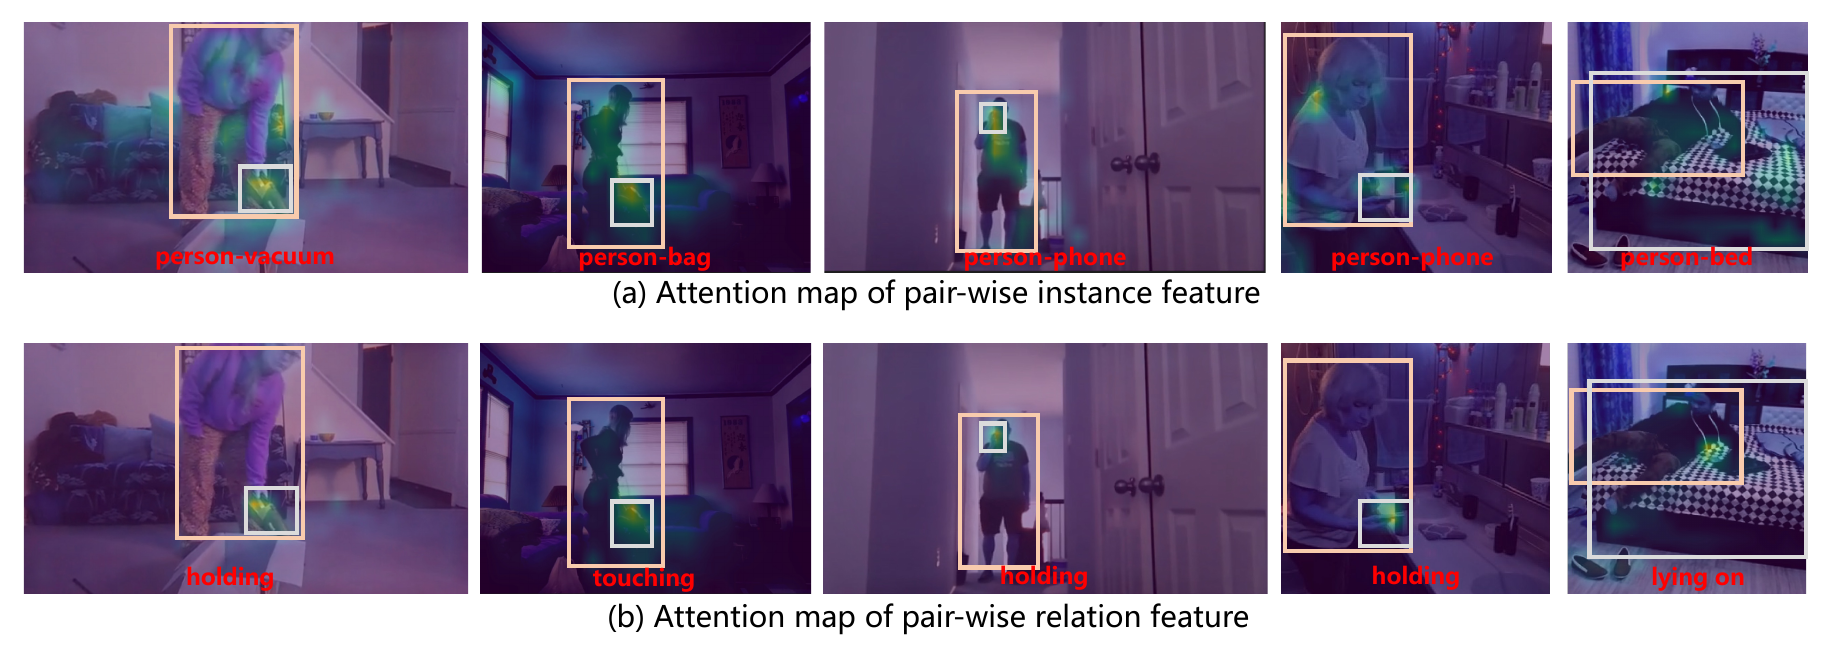}
    \caption{Visualization of attention maps of pair-wise instance feature and pair-wise relation feature.}
\label{fig:supp_visual_attn}
\end{figure*}
