# Supplementary material for: OED: Towards One-stage End-to-End Dynamic Scene Graph Generation
Source: arXiv:2405.16925 source file (2024-05-27)
Supplement: Supplementary file 4 [file supp_fig3_scene_graph.tex]

\begin{figure*}[htpb]
    \includegraphics[width=\linewidth]{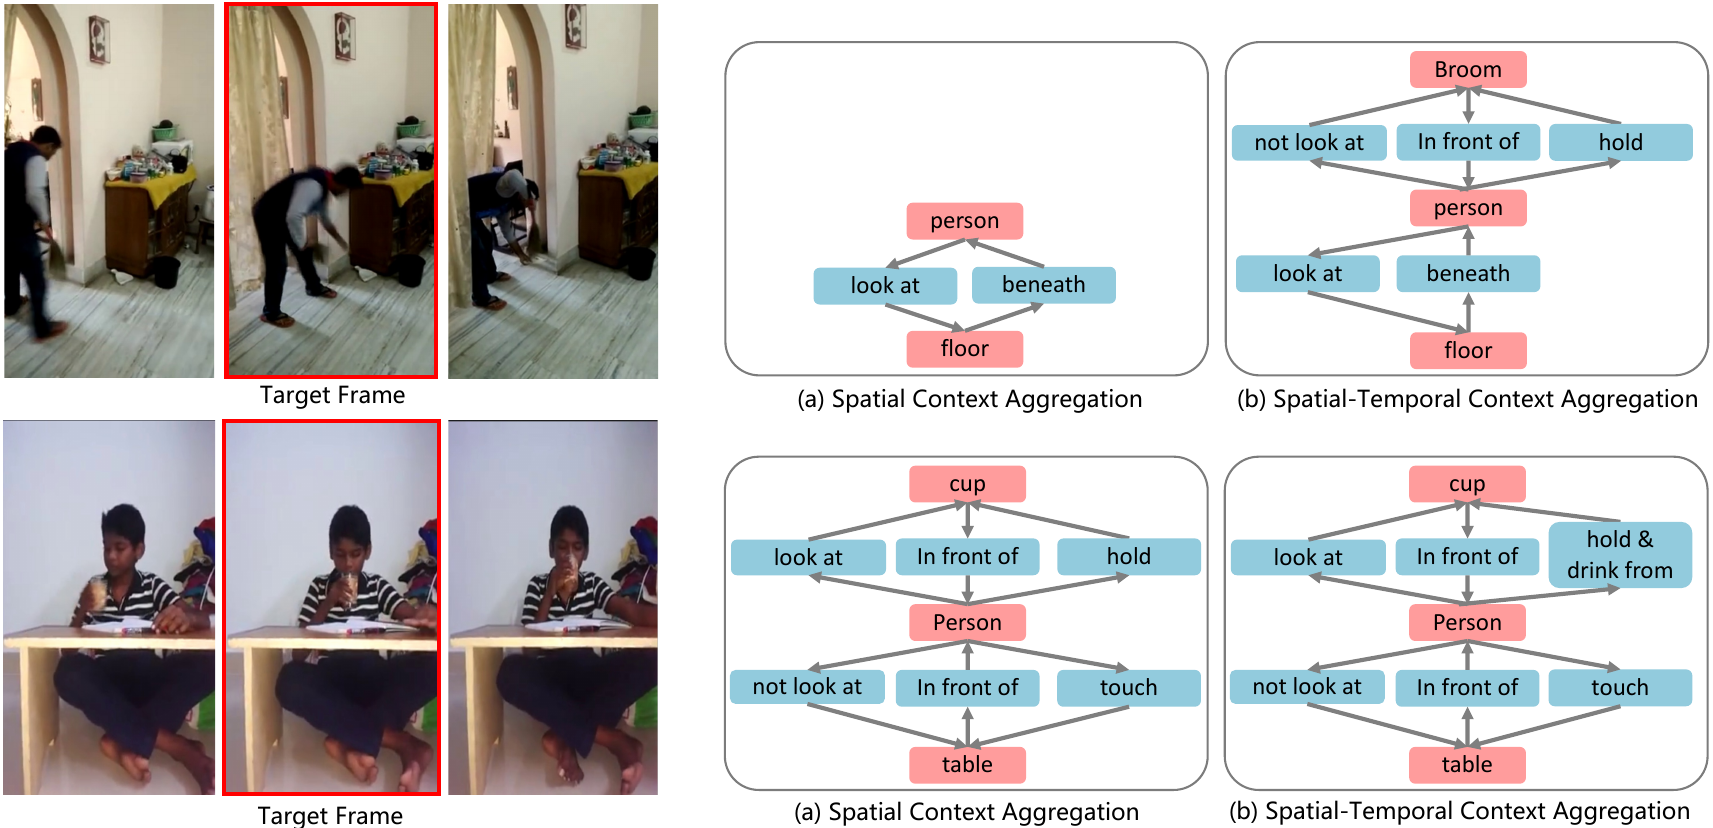}
    \caption{Part of predictions of our Spatial Context Aggregation and Spatial-Temporal Context Aggregation under \textit{with constraint} setting, which match with ground truth.}
\label{fig:supp_scene_graph}
\end{figure*}
