# Supplementary material for: OED: Towards One-stage End-to-End Dynamic Scene Graph Generation
Source: arXiv:2405.16925 source file (2024-05-27)
Supplement: Supplementary file 5 [file x_supp_long-tail.tex]

\begin{table*}[h!]
\captionsetup{font=footnotesize}
% \fontsize{40.5}{13.8}\selectfont

% \setlength{\abovecaptionskip}{0cm} % 调整间距
% \setlength{\belowcaptionskip}{-0.4cm}
\Huge
\centering
\caption{Performance comparison under both Recall and Mean Recall Metrics and Head-body-tail classes with mR@50.}
\resizebox{\textwidth}{!}{
\begin{tabular}{c ccc|ccc|ccc | ccc|ccc|ccc}
\toprule
  & \multicolumn{9}{c|}{With Constraint} & \multicolumn{9}{c}{No Constraints} \\ 
  \cmidrule(lr){2-10} \cmidrule(lr){11-19}
  Method
    &R@10 &R@20 &R50 &mR@10 &mR@20 &mR50  &Head &Body &Tail &R@10 &R@20 &R50 &mR@10 &m20 &mR50  &Head &Body &Tail\\
% \midrule
\midrule

STTran~\cite{cong2021spatial}	&25.2 &34.0 &\underline{36.9} &16.5 &20.8 &22.2 &\underline{39.00} &25.53 &12.78  &24.5 &36.1 &\underline{48.8} &20.9 &29.6 &39.1 &\underline{45.39} &52.32 &26.67 \\
DSG-DETR~\cite{feng2023exploiting} &\underline{30.4} &\underline{34.9} &36.0 &18.0 &21.3 &22.0 &37.91 &\underline{25.84} &12.62 &\underline{32.3} &\underline{40.9} &48.2 &23.6 &30.1 &36.5 &44.76 &\underline{52.65} &21.09 \\
TEMPURA~\cite{nag2023unbiased} &28.0 &33.3 &34.8 &\underline{18.4} &\underline{22.5} &\underline{23.6} &36.53 &23.79 &\underline{18.15} &29.8 &38.0 &46.3 &\underline{24.5} &\underline{33.8} &\underline{43.6} &42.50 &50.66 &\underline{38.86} \\
Ours &\textbf{33.5} &\textbf{40.9} &\textbf{48.9} &\textbf{20.9} &\textbf{26.9} & \textbf{32.9} &\textbf{51.44} &\textbf{36.38} &\textbf{22.72} &\textbf{35.3} &\textbf{44.0} &\textbf{51.8} &\textbf{26.3} &\textbf{39.5} &\textbf{49.5} &\textbf{48.75} &\textbf{56.12} &\textbf{44.89} \\

\bottomrule
\end{tabular}
}
\label{tab:supp_long_tail}
% \vspace{-13pt}
\end{table*}
